# Supplementary material for: Symbolic Visual Reinforcement Learning: A Scalable Framework with Object-Level Abstraction and Differentiable Expression Search
Source: arXiv:2212.14849 source file (2022-12-30)
Supplement: Supplementary file 1 [file _NeurIPS22__symrel_v1-supple.pdf]

---

# Understanding Visual Reinforcement Learning Via Symbolic Regression (Appendix)

---

Anonymous Author(s)

Affiliation

Address

email

## 1 A What’s in the supplementary materials

2 In the supplementary materials, we put the sampled implementations (full implementations will be  
3 open-sourced upon acceptance), and three video demonstrations:

- 4 • The *denoised-action-distribution.mp4* shows the actions for the original DRL and the  
5 distilled symbolic expression distilled from the denoised dataset in some environments.
- 6 • The *transferrability.mp4* compared the different transferability for the distilled symbolic  
7 expression and the DRL agent.
- 8 • The *tree-evaluation.mp4* uses the tree structure to visualize the action of the distilled  
9 symbolic equation.

## 10 B Distilled Policies Under Different Failure Modes

11 In this section we compared the different distilled symbolic policies under different types of failures.  
12 As the symbolic policy contains object detection, geometric operators and numerical operators, we  
13 include ablation studies for these components by simulating the failures of these modules. The  
14 ablation results for the object detection is displayed in Table. 3 in the main text. For the geometric  
15 and numerical operators, we simulate the failure modes by removing certain important operators  
16 from the search space and compare the resulting symbolic expressions and their performances. We  
17 still take the CircusCharlie environment as our case study. We dropped one “critical” geometric  
18 operator (*has\_intersection*), one important numerical operator (*is*( $x < y$ )). The performances  
19 are provided in Table. 4 in the main text. The resulting tree structures are in Figure 1.

## 20 C Details of optical flow based object detection

21 Since in most retro environments, the image styles are simple, where the backgrounds are nearly  
22 fixed and the objects share similar patterns. Therefore, we take the optical flow as a simplified object  
23 detection module.

24 We first segment out the object list from template matching, then estimate the velocity using the  
25 pretrained FlowNet [1], and get the speed via the average optical flow of detected objects. The classes  
26 of the objects are obtained based on the shape in the predefined templates.

## 27 D More Examples of distilled symbolic policy

28 A plenty of environments are found to be viable for symbolic distillation (approximately 85% of  
29 1000+ gym retro environments). A sampled list of such environments are put in Appendix E.

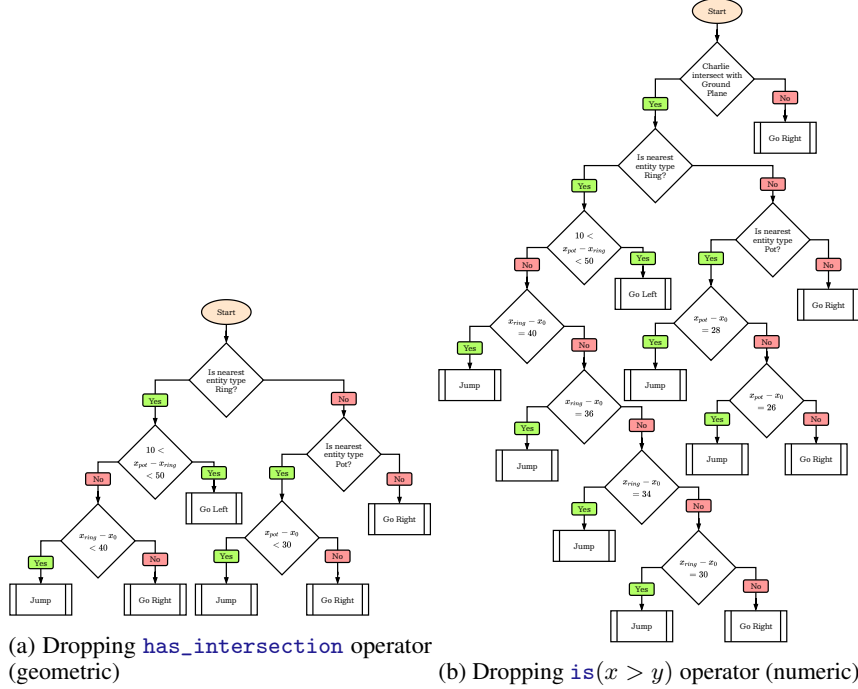

Figure 1: Missing operators from operator search space of the CircusCharlie environment.

We check the learned symbolic operators in the tree nodes, and re-write them as interpretable symbolic tree policy. The results are plotted in Fig. 5, Fig. 3, Fig 6, Fig 2, Fig 4, and Fig 7.

## E Examples of Retro-Env List That One-Frame Symbolic Distillation Can Work Well

After checking the underlying logics and evaluated the possible strategies of gym-retro environments, a plenty of them are found to be solvable by our symbolic policy distillation. Several examples include: 8Eyes-Nes, 1942-Nes, BadDudes-Nes, BioSenshiDanIncreaserTonoTatakai-Nes, BreakThru-Nes, BubbleBobble-Nes, CodeNameViper-Nes, FrontLine-Nes, GhostsnGoblins-Nes, KidIcarus-Nes, KidNikiRadicalNinja-Nes, Parodius-Nes, RoboccoWars-Nes, Sansuu5And6NenKeisanGame-Nes, Seicross-Nes, SonSon-Nes, Tennis-Atari2600, TwinEagle-Nes, ViceProjectDoom-Nes, Xexyz-Nes, MysteryQuest-Nes. The screenshots for them are displayed in Fig. 8.

## F Quantized Fitting Ability

We compare the fitting ability of the distilled the symbolic policy and the original DRL policy via comparing their action distributions on the behavior dataset generated by the DRL model. The steps to generate metrics are as follows.

1. Create dataset of frames from 16 full games played by a PPO model with corresponding input-output pairs.
2. Replay each step by a distilled agent and record action taken by iterating through the dataset created.
3. Create confusion matrix of results, then other evaluation metrics are instantly available through the confusion matrix.

In the pong environment, the confusion matrix results are displayed in Figure 9.

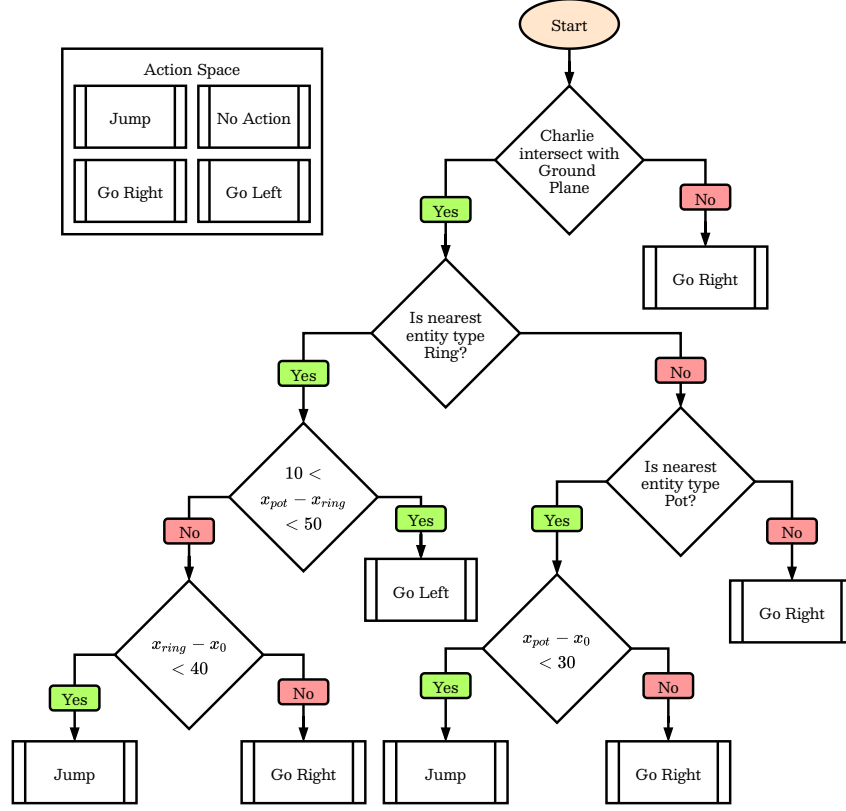

Figure 2: Distilled policy for CircusCharlie-Nes

## References

- [1] Eddy Ilg, Nikolaus Mayer, Tonmoy Saikia, Margret Keuper, Alexey Dosovitskiy, and Thomas Brox. FlowNet 2.0: Evolution of optical flow estimation with deep networks. In *Proceedings of the IEEE conference on computer vision and pattern recognition*, pages 2462–2470, 2017.

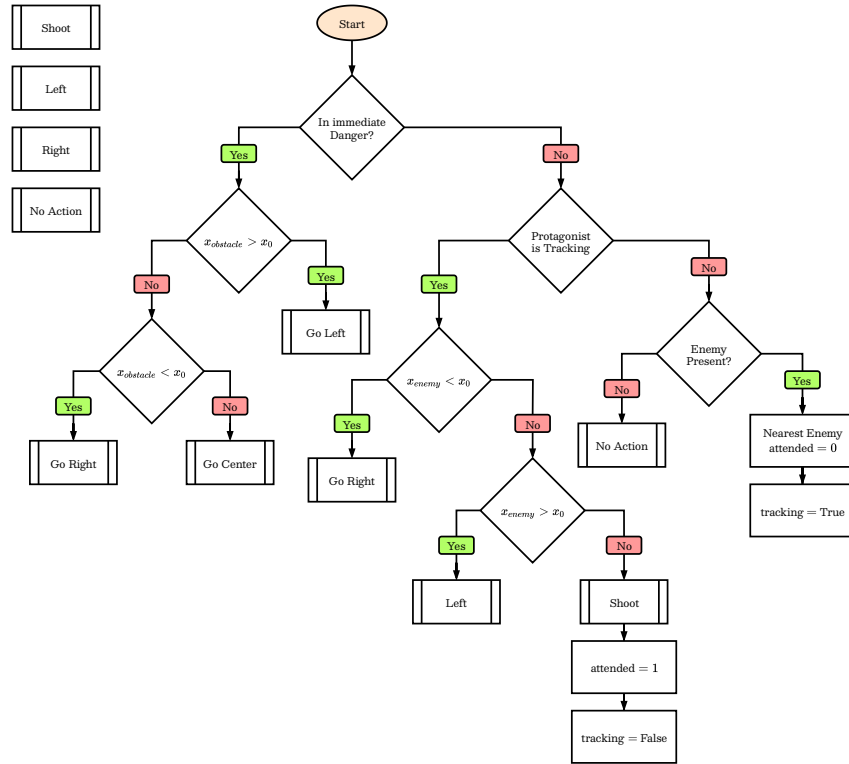

Figure 3: Distilled policy for Airstriker-Genesis

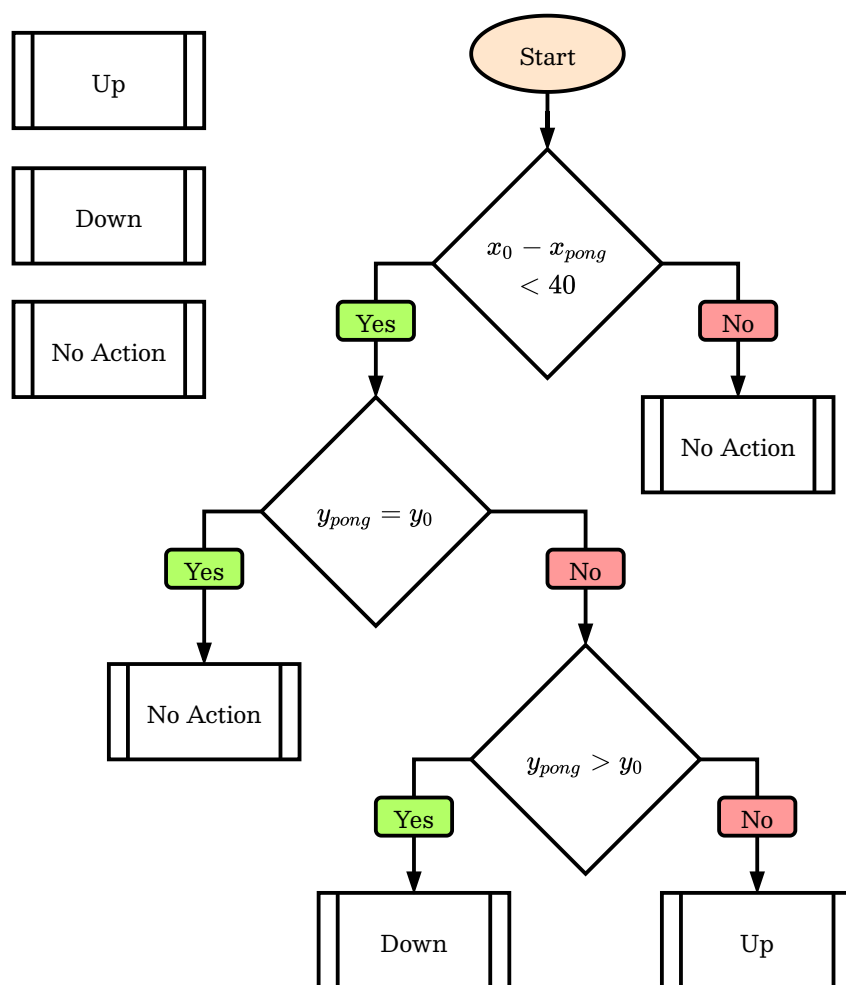

Figure 4: Distilled policy for Pong-Atari2600

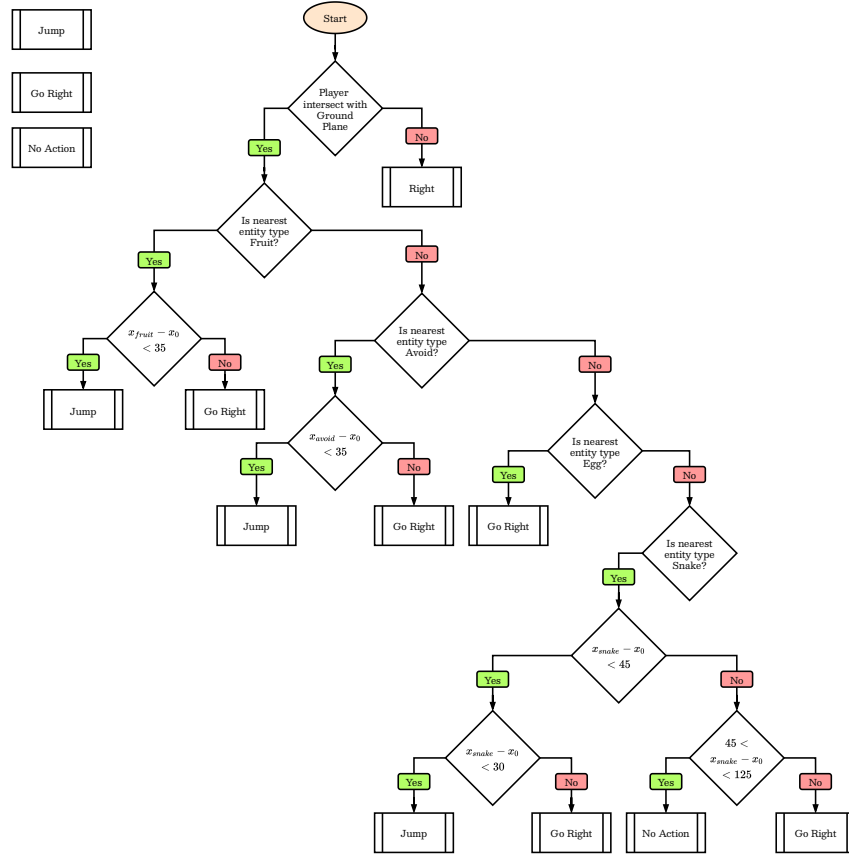

Figure 5: Distilled policy for AdventureIsland3-Nes

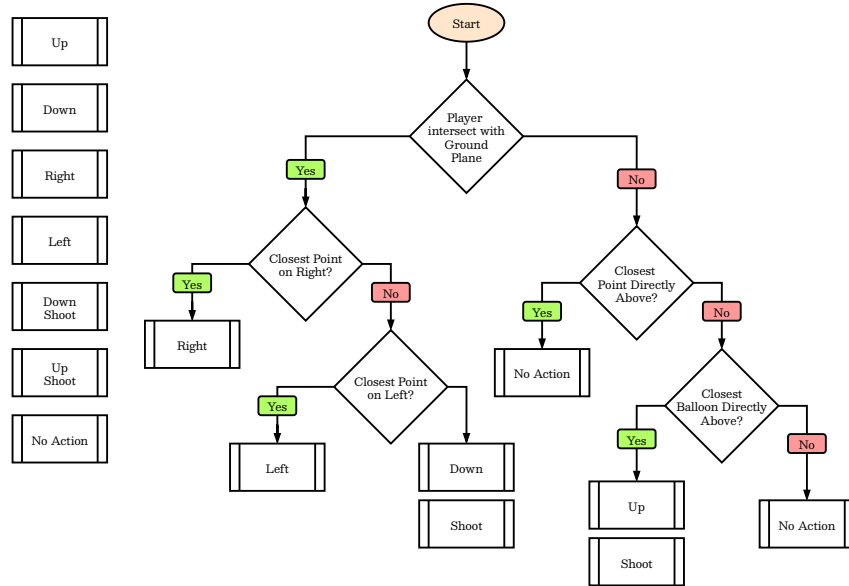

Figure 6: Distilled policy for AstroRoboSasa-Nes

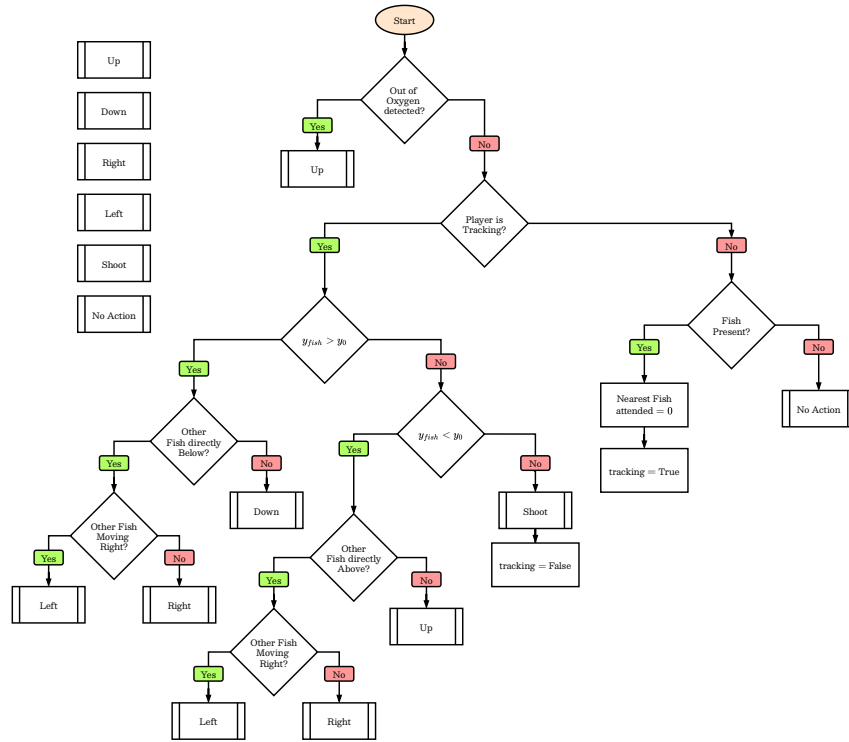

Figure 7: Distilled policy for Seaquest-Atari2600

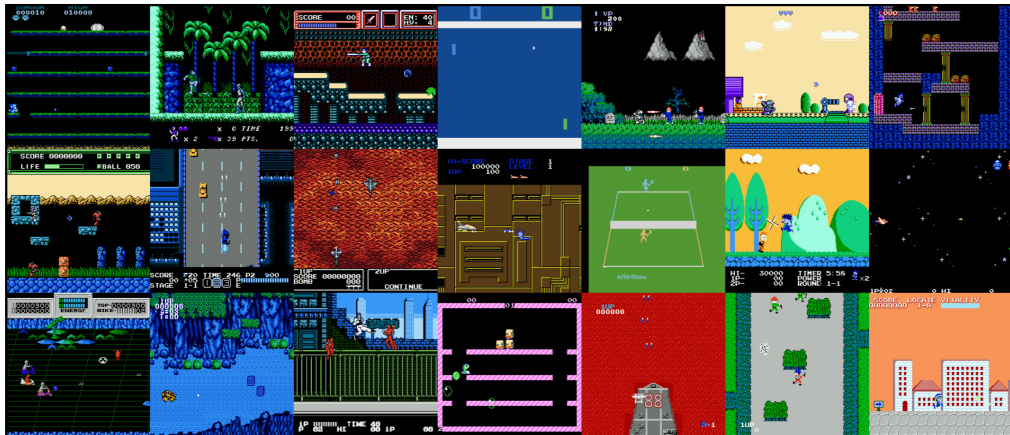

Figure 8: Several environments found to be viable for symbolic distillation.

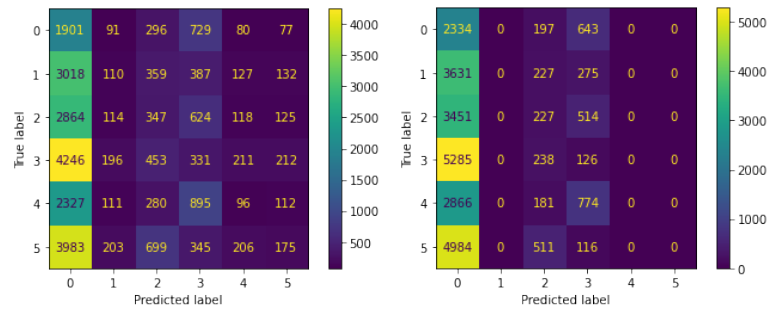

(a) Pong on full dataset

(b) Pong on denoised dataset

Figure 9: Confusion matrices of predictions.
