# Supplementary material for: Symbolic Visual Reinforcement Learning: A Scalable Framework with Object-Level Abstraction and Differentiable Expression Search
Source: arXiv:2212.14849 source file (2022-12-30)
Supplement: Supplementary file 2 [file _NeurIPS22__symrel_v2-supple.pdf]

---

# Appendix – Differentiable Symbolic Architecture Search: Less Handcrafting and Better Scalability For Symbolic Visual Reinforcement Learning

---

Anonymous Author(s)

Affiliation

Address

email

## A Appendix

Through our Supplementary Appendix, we comment and analyze our model performance on the various tasks as discussed in our main text, both qualitatively and quantitatively. We have also included sampled python implementations of our proposed method under a separate folder in our zip. Our codes will be open-sourced upon acceptance.

### A.1 Ablation Study On Sub-optimal Unsupervised Object Detection

As the our generated symbolic rule is quite reliant on the success of the object detection algorithm and timely identification of key entities, one reasonable issue is whether the symbolic rule will become unreliable if the OD module fails. Therefore, in this section, we take a look at two case studies – firstly, we test out various levels of suboptimal object detectors and measure the drop in performances of trained symbolic agents, and secondly, test the OD module trained on one environment by deployed on an entirely unseen but similar environment.

#### A.1.1 Handling Deficient Object Detection

As a part of our first case study, we emulate a badly performing object detector by using intermediate training checkpoints of a fully trained object detector and compare its accuracy and rewards with its fully trained counterparts. Specifically, we sample checkpoints of SPACE at 30%, 50%, and 80% of its training. We then retrain the D-SAS on each of their outputs and compare their performances with a 100% trained OD agent on the same. In Table 1, we calculate the Average Precision for an IoU threshold of 50% with respect to a ground-truth generated through a handcrafted template-matching based approach. We see that the rewards still maintain an *acceptable* range does not lead to the whole-scale collapse of the algorithm.

| Intermediate OD Checkpoint | OD Avg. Precision | Reward |
|----------------------------|-------------------|--------|
| 30% trained                | 41.66             | 1091   |
| 50% trained                | 68.21             | 2271   |
| 80% trained                | 77.94             | 2681   |

Table 1: Checkpoints of OD taken from the middle of training.

#### A.1.2 Handling Unseen Environments

Our second case study covers the scenario when an object detection is not performing well on the environment it was trained on. We test the pipeline on an environment which is entirely different from

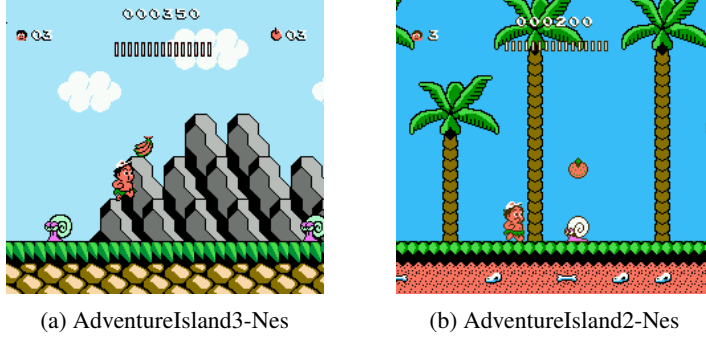

Figure 1: Visual comparison of the environments involved in OD transfer ablation.

one it was trained on. For this, we first train SPACE, our object detection module on AdventureIsland3-Nes, a retro-gym game and train D-SAS on it till convergence. Then, we directly try using that object detector on AdventureIsland2-Nes, an unseen but mildly visually similar environment. We then retrain our D-SAS algorithm based on the objects detected in this environment by the old object detector and contrast their performance.

| Environment          | OD Avg. Precision | Reward |
|----------------------|-------------------|--------|
| AdventureIsland3-Nes | 79.25             | 2717   |
| AdventureIsland2-Nes | 52.21             | 1623   |

Table 2: OD Trained on AdventureIsland3-Nes transferred to AdventureIsland2-Nes.

In conclusion, the results show that acceptable performance can be enjoyed by our method even during failure cases of object detection. On the other hand, even though the object detector is unable to retain its accuracy post-transfer, our method is capable of working with those outputs and is able to regress a robust rule and achieves satisfactory rewards.

## A.2 Visualization of Resultant Policies

In this section, we visualize the policies resultant from the Differentiable Symbolic Architecture Search for different environments. We also provide results on a few other Visual RL environments in table 3. We also visualize a few of their policies in the form of symbolic trees in Figure 2, Figure 3, and Figure 5.

| Environment        | D-SAS Reward | PPO Reward |
|--------------------|--------------|------------|
| CircusCharlie-Nes  | 3549         | 4580       |
| AstroRoboSasa-Nes  | 1256         | 966        |
| Seaquest-Atari2000 | 191          | 208        |
| Airstriker-Genesis | 421          | 383        |

Table 3: Additional results of D-SAS on visual-based environments.

## A.3 Erroneous Object Splitting

In a few instances of object detection, the SPACE algorithm tends to split a single object into multiple smaller parts as seen in Figure 4. It could be a flaw of the patch-based processing that SPACE employs. Although it can be prevented by careful hyper-parameter optimization of the boundary loss coefficients and bounding box sizes of the object detector, we do not attempt to “overfit” the hyper parameters towards any single environment in our setting as to maintain the notion of a truly end-to-end generalized framework with *no handcrafting required*.

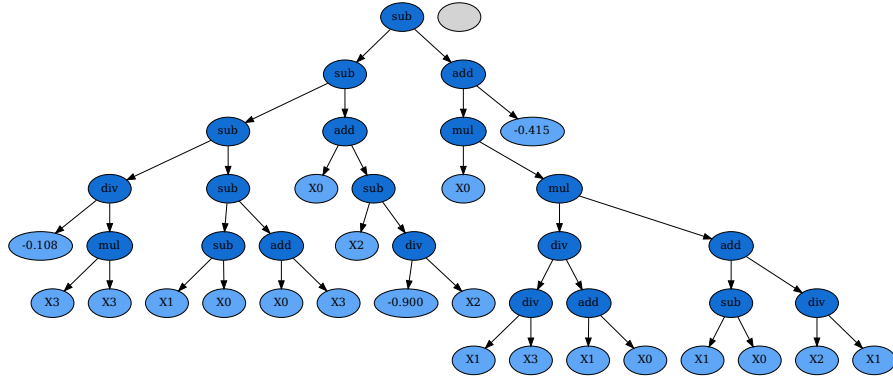

Figure 2: Visualization of a trained D-SAS policy for the Pong-Atari2600 environment

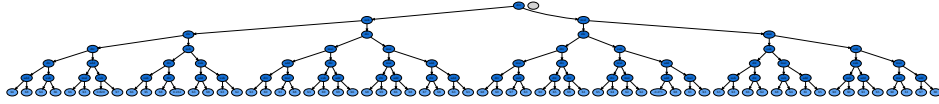

Figure 3: Visualization of a trained D-SAS policy for the Seaquest-Atari2600 environment

46 Despite such erroneous detection, D-SAS is infact capable of regressing robust rules for these  
 47 environments as seen in our additional environment results Table 3 and Figure 5. This is as the policy  
 48 actually takes into account just any one of the detected parts (so long as atleast one part is detected),  
 49 and determines the rule, therefore being able to workaround poor detections.

#### 50 A.4 Qualitative Demonstrations of Object Detection

51 We provide numerous qualitative results of the object detection in Figure 6 for visualization purposes.  
 52 It is observed that even on very diverse settings and visual scenarios being a combination of dynamic  
 53 objects, the OD framework is capable of detecting objects well.

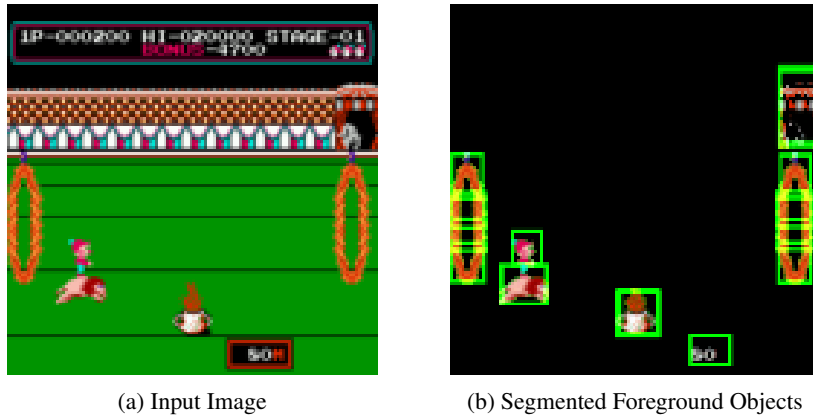

Figure 4: Erroneous Object Splitting in the case of “Fire-Ring” and “Charlie” in CircusCharlie-Nes. Observe that the ring gets broken up into four pieces and Charlie and his Lion get separated into two entities.

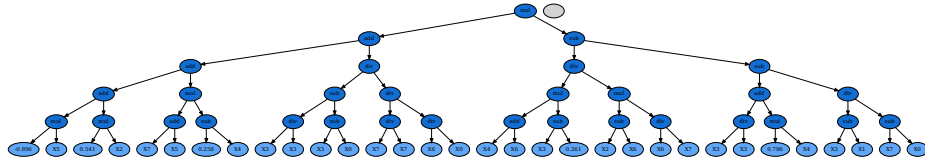

Figure 5: Visualization of a trained D-SAS policy for the CircusCharlie-Nes environment

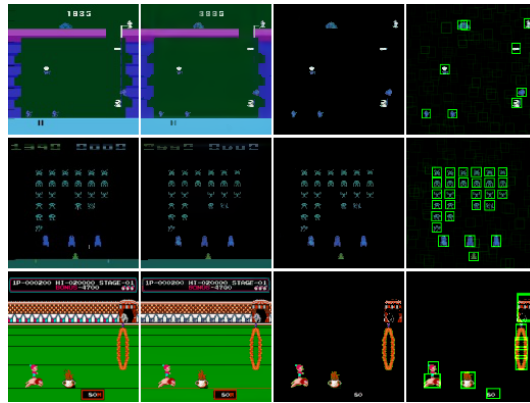

Figure 6: Qualitative demonstrations of SPACE on a selection of Visual-RL environments.
